# Supplementary material for: Counting independent sets in cubic graphs of given girth
Source: arXiv:1611.01474 ancillary file (2018-04-11)
Supplement: Supplementary file 1 [file CubicCalculations.pdf]

# Counting independent sets in cubic graphs of given girth

## *Auxiliary calculations*

Guillem Perarnau, Will Perkins

---

### Instructions

1. Begin by running “Evaluate Initialization Cells” from the “Evaluation” menu.
2. The cells with gray background define the functions from Section 5.
3. The cells with the green background define the configurations.
4. The cells with the yellow background compute and verify the claims of the paper.

---

### Preliminary Functions

We define the partition function  $P_{H_{3,6}}(\lambda)$  and occupancy fraction  $\alpha_{H_{3,6}}(\lambda)$  of the Heawood graph.

$$\begin{aligned} \text{In[1]:= } \text{PH36}[\lambda\_]&:= 1 + 14 \lambda + 70 \lambda^2 + 154 \lambda^3 + 147 \lambda^4 + 56 \lambda^5 + 14 \lambda^6 + 2 \lambda^7; \\ \alpha_{\text{H36}}[\lambda\_]&:= \frac{\lambda (14 + 140 \lambda + 462 \lambda^2 + 588 \lambda^3 + 280 \lambda^4 + 84 \lambda^5 + 14 \lambda^6)}{14 (1 + 14 \lambda + 70 \lambda^2 + 154 \lambda^3 + 147 \lambda^4 + 56 \lambda^5 + 14 \lambda^6 + 2 \lambda^7)}; \end{aligned}$$

We define the partition function  $P_{P_{5,2}}(\lambda)$  and occupancy fraction  $\alpha_{P_{5,2}}(\lambda)$  of the Petersen graph.

$$\begin{aligned} \text{In[3]:= } \text{PP52}[\lambda\_]&:= 1 + 10 \lambda + 30 \lambda^2 + 30 \lambda^3 + 5 \lambda^4; \\ \alpha_{\text{P52}}[\lambda\_]&:= \frac{\lambda (10 + 60 \lambda + 90 \lambda^2 + 20 \lambda^3)}{10 (1 + 10 \lambda + 30 \lambda^2 + 30 \lambda^3 + 5 \lambda^4)}; \end{aligned}$$

We will represent a configuration as a list of three lists :  $\{V_2, E_{12}, E_{22}\}$ ,  $V_2$  is the list of externally uncovered 2nd neighbors,  $E_{12}$  is the list of edges from 1st to 2nd neighbors, and  $E_{22}$  is the list of edges within  $V_2$ . We use  $\{1, 2, 3\}$  to represent 1st neighbors of  $v$  and  $\{4, 5, 6, 7, 8, 9\}$  to represent 2nd neighbors.

Take for instance the configuration:  $C = \{\{4, 5, 6\}, \{\{1, 4\}, \{1, 5\}, \{2, 6\}, \{2, 7\}, \{3, 8\}, \{3, 9\}\}, \{\{4, 6\}\}\}$ .

Here there are 3 externally uncovered 2nd neighbors, labeled 4, 5 and 6. The 2nd neighbors with labels 7, 8 and 9 are covered by some occupied external neighbor. The 1st neighbors are labeled 1, 2 and 3. There are edges from 1 to 4 and 5; from 2 to 6 and 7; and from 3 to 8 and 9, though in this case the edges to 7, 8 and 9 are irrelevant since they are covered. Finally there is a single edge between 4 and 6 between 2nd neighbors.

The **Neighbors** function takes an edge list and a label 1, 2, or 3 and returns the vertices in the 2nd neighborhood that adjoin the given vertex

```
Neighbors[E12_, j_] := Flatten[Table[If[e[[1]] == j, e[[2]], {}], {e, E12}]];
```

For example,

```
Neighbors[{{1, 4}, {1, 5}, {2, 6}, {2, 7}, {3, 8}, {3, 9}}, 2]
{6, 7}
```

Next we define functions that will compute the partition functions, the alpha function, and the gamma functions for each configuration.

To each function we pass  $\lambda$  as well as the configuration CC represented as above, e.g.  $CC = \{V_2, E_{12}, E_{22}\}$ .

Compute the contribution to the partition function when  $v$  in  $I$  and the subset  $S2$  of 2nd neighbors is in  $I$ . (eq (11))

```
ZvOcS[CC_, λ_, S2_] := (V2 = CC[[1]]; E22 = CC[[3]];
  If[SubsetQ[V2, S2], 1, 0] *
  λ^(1 + Length[S2]) * Product[If[SubsetQ[S2, e], 0, 1], {e, E22}]];
```

Compute the contribution to the partition function of all  $I$  such that  $v$  in  $I$  by summing over all possible subsets  $S2$  of the externally uncovered 2nd neighborhood.

```
ZvOc[CC_, λ_] := (V2 = CC[[1]];
  Sum[ZvOcS[CC, λ, S2], {S2, Subsets[V2]}]);
```

Compute the contribution to the partition function of  $I$  such that  $v$  not in  $I$ , the subset  $S1$  of 1st neighbors is in  $I$ , and the subset  $S2$  of 2nd neighbors is in  $I$ . (eq (12))

```
ZvUnOcS[CC_, λ_, S1_, S2_] := (V2 = CC[[1]];
  E12 = CC[[2]]; E22 = CC[[3]];
  If[SubsetQ[V2, S2], 1, 0] * λ^(Length[S1] + Length[S2]) * Product[If[SubsetQ[Union[
    S1, S2], e], 0, 1], {e, E12}] * Product[If[SubsetQ[S2, e], 0, 1], {e, E22}]];
```

Compute the contribution to the partition function of all  $I$  such that  $v$  not in  $I$  by summing over all possible subsets  $S1$  and  $S2$  of the 1st and 2nd neighborhoods:

```
ZvUnOc[CC_, λ_] := (V2 = CC[[1]];
  Sum[Sum[ZvUnOcS[CC, λ, S1, S2], {S1, Subsets[{1, 2, 3]}]}, {S2, Subsets[V2]}];
```

Compute the partition function by adding contributions when  $v$  in  $I$  and  $v$  not in  $I$ . (eq (13))

```
ZZ[CC_, λ_] := ZvOc[CC, λ] + ZvUnOc[CC, λ];
```

Compute  $\alpha_{C,v}(\lambda)$ . (eq (14))

```
AlpV[CC_, λ_] := ZvOc[CC, λ] / ZZ[CC, λ];
```

Compute  $\gamma_t^v(C)$ , that is the probability that  $v$  sees  $t$  occupied neighbors, by summing contributions to the partition function over all subsets  $S1$  and  $S2$  and checking the size of  $S1$  is  $t$ , then dividing by the partition function. We can restrict ourselves to summing over  $I$  s.t.  $v$  not in  $I$ ; if  $t=0$  then we multiply by an additional  $(1+\lambda)$  factor since  $v$  can be in as well. (eq (15))

```
GamV[CC_, λ_, t_] := (V2 = CC[[1]];
  If[t == 0, (1 + λ), 1] * Sum[Sum[If[Length[S1] == t, 1, 0] * ZvUnOcS[CC, λ, S1, S2],
    {S1, Subsets[{1, 2, 3]}]}, {S2, Subsets[V2]}] / ZZ[CC, λ];
```

Compute  $\gamma_t^u(C)$ , that is the average probability that a random neighbor  $u$  of  $v$  sees  $t$  occupied neighbors, by first summing over the 3 first neighbors, then summing contributions to the partition function over all subsets  $S1$  and  $S2$  and checking the number of occupied neighbors of  $u$  is  $t$ , then dividing by the partition function. We distinguish two cases: if  $t=0$ , then we restrict to independent sets  $I$  such that  $v$  not in  $I$  and such that no occupied 2nd neighbors of  $v$  are also neighbors of  $u$ ; if  $t \geq 1$  then we have two cases, if  $v$  is in  $I$ , then we restrict to subsets  $S2$  with  $t-1$  occupied 2nd neighbors of  $v$  that are neighbors of  $u$ , and if  $v$  not in  $I$ , then we restrict to subsets  $S2$  with  $t$  occupied 2nd neighbors of  $v$  that are neighbors of  $u$ . (eq (16), (17))

```
GamU[CC_, λ_, t_] := (V2 = CC[[1]]; E12 = CC[[2]];
  1 / 3 / ZZ[CC, λ] * Sum[If[t == 0, Sum[Sum[If[Length[Intersection[Neighbors[E12, j],
    S2]] == 0, 1, 0] * ZvUnOcS[CC, λ, S1, S2], {S1, Subsets[{1, 2, 3]}]},
    {S2, Subsets[V2]}], Sum[If[Length[Intersection[Neighbors[E12, j], S2]] ==
    t - 1, 1, 0] * ZvOcS[CC, λ, S2], {S2, Subsets[V2]}] + Sum[Sum[
    If[Length[Intersection[Neighbors[E12, j], S2]] == t, 1, 0] * ZvUnOcS[CC, λ,
    S1, S2], {S1, Subsets[{1, 2, 3]}]}, {S2, Subsets[V2]}], {j, 1, 3}]]];
```

## List of Configurations

A list of all 207 configurations in  $C_4$ . An extra blank line is added when  $E_{12}$  changes. See appendix B for the drawing of each configuration.

In[14]:=

```
CONFIGURATIONS4 = {
  {{4, 5, 6, 7, 8, 9}, {{1, 4}, {1, 5}, {2, 6}, {2, 7}, {3, 8}, {3, 9}}, {}},
```

[illegible]

[illegible]

[illegible]

```
{ {4, 6}, { {1, 4}, {1, 5}, {2, 5}, {2, 6}, {3, 5}, {3, 6}}, { {4, 6}}},
{ {4, 5}, { {1, 4}, {1, 5}, {2, 4}, {2, 5}, {3, 4}, {3, 5}}, {}},
{ {4}, { {1, 4}, {1, 5}, {2, 4}, {2, 5}, {3, 4}, {3, 5}}, {}},
{ {}, { {1, 4}, {1, 5}, {2, 4}, {2, 5}, {3, 4}, {3, 5}}, {}}};
```

```
In[15]:= Length[CONFIGURATIONS4]
```

```
Out[15]= 207
```

We form the subset of configurations with 6 distinct 2nd neighbors. These appear in appendix B.1. This is a superset of  $C_5$  so it suffices to show that the slack function is non-negative on all of these.

```
In[16]:= CONFIGURATIONS5 = Table[CONFIGURATIONS4[[i]], {i, 1, 79}];
```

## Theorem 5

Here we define the SLACK function (equation (6)) we use to prove Theorem 5.

```
In[17]:= Slack5[λ_, Δ0_, Δ1_, Δ2_, CC_] :=
  αH36[λ] - A1pV[CC, λ] + Δ0 * ( GamV[CC, λ, 0] - GamU[CC, λ, 0] ) +
  Δ1 * ( GamV[CC, λ, 1] - GamU[CC, λ, 1] ) + Δ2 * ( GamV[CC, λ, 2] - GamU[CC, λ, 2] )
```

We define the dual variables as in Claim 8.

```
In[18]:= Lam50[λ_] := - ( (3 + 27 λ + 94 λ^2 + 139 λ^3 + 20 λ^4 - 139 λ^5 - 124 λ^6 - 45 λ^7 - 9 λ^8 - λ^9) /
  (2 + 31 λ + 183 λ^2 + 532 λ^3 + 826 λ^4 + 707 λ^5 + 343 λ^6 + 102 λ^7 + 20 λ^8 + 2 λ^9) );
Lam51[λ_] := - ( (3 + 24 λ + 73 λ^2 + 99 λ^3 + 25 λ^4 - 63 λ^5 - 55 λ^6 - 15 λ^7 - λ^8) /
  ( (2 + λ) (1 + 14 λ + 70 λ^2 + 154 λ^3 + 147 λ^4 + 56 λ^5 + 14 λ^6 + 2 λ^7) ) );
Lam52[λ_] := - ( (3 + 27 λ + 94 λ^2 + 160 λ^3 + 132 λ^4 + 46 λ^5 + 3 λ^6 - λ^7) /
  ( (2 + λ) (1 + 14 λ + 70 λ^2 + 154 λ^3 + 147 λ^4 + 56 λ^5 + 14 λ^6 + 2 λ^7) ) );
```

We define the scaled slack function as in equation (8).

```
In[21]:= F5[λ_, Δ0_, Δ1_, Δ2_, CC_] := 3 * (λ + 2) * PH36[λ] * ZZ[CC, λ] * Slack5[λ, Δ0, Δ1, Δ2, CC];
```

We compute the scaled slack function on each configuration and compute its coefficients as a polynomial in  $\lambda$ , as well as reporting if it is identically 0.

```
CoefListTable0 = Table[{}, {i, 1, Length[CONFIGURATIONS5]}];
For[i = 1, i < Length[CONFIGURATIONS5] + 1, i++, scaledSlack =
  Simplify[ F5[λ, Lam50[λ], Lam51[λ], Lam52[λ], CONFIGURATIONS5[[i]]] ];
  CoefListTable0[[i]] = CoefficientList[scaledSlack, λ];
  If[CoefListTable0[[i]] == {}, Print["Config: ", i, " identically 0"]];
  (*Print["Config: ", i, " Scaled Slack: ", CoefficientList[scaledSlack, λ]]*)
];
```

```
Config: 1 identically 0
```

```
Config: 7 identically 0
```

```
Config: 9 identically 0
```

```
Config: 10 identically 0
```

```
Config: 19 identically 0
```

Confirm non-negative coefficients, and print all coefficients as an array.

```
Print["Minimum coefficient in  $\lambda$ : ", Min[Flatten[CoefListTable0]]]
TableForm[CoefListTable0]
```

Minimum coefficient in  $\lambda$ : 0

|   |   |   |   |   |    |     |     |      |      |      |     |     |   |
|---|---|---|---|---|----|-----|-----|------|------|------|-----|-----|---|
| 0 | 0 | 0 | 0 | 0 | 6  | 66  | 286 | 626  | 762  | 528  | 200 | 36  | 2 |
| 0 | 0 | 0 | 0 | 0 | 12 | 138 | 604 | 1273 | 1428 | 899  | 316 | 57  | 4 |
| 0 | 0 | 0 | 0 | 0 | 6  | 57  | 212 | 391  | 384  | 197  | 46  | 3   |   |
| 0 | 0 | 0 | 0 | 0 | 9  | 84  | 303 | 523  | 458  | 209  | 47  | 4   |   |
| 0 | 0 | 0 | 0 | 0 | 12 | 90  | 252 | 337  | 236  | 88   | 16  | 1   |   |
| 0 | 0 | 0 | 0 | 0 | 0  | 3   | 20  | 41   | 30   | 11   | 2   |     |   |
| 0 | 0 | 0 | 0 | 0 | 6  | 75  | 360 | 861  | 1140 | 859  | 354 | 69  | 4 |
| 0 | 0 | 0 | 0 | 0 | 12 | 114 | 424 | 782  | 768  | 394  | 92  | 6   |   |
| 0 | 0 | 0 | 0 | 0 | 18 | 165 | 586 | 1005 | 886  | 407  | 92  | 8   |   |
| 0 | 0 | 0 | 0 | 0 | 9  | 111 | 513 | 1141 | 1354 | 887  | 315 | 56  | 4 |
| 0 | 0 | 0 | 0 | 0 | 9  | 81  | 283 | 482  | 428  | 198  | 45  | 4   |   |
| 0 | 0 | 0 | 0 | 0 | 12 | 93  | 272 | 378  | 266  | 99   | 18  | 1   |   |
| 0 | 0 | 0 | 0 | 0 | 6  | 78  | 354 | 709  | 680  | 330  | 78  | 7   |   |
| 0 | 0 | 0 | 0 | 0 | 0  | 6   | 40  | 82   | 60   | 22   | 4   |     |   |
| 0 | 0 | 0 | 0 | 0 | 12 | 144 | 672 | 1573 | 2028 | 1444 | 552 | 105 | 8 |
| 0 | 0 | 0 | 0 | 0 | 18 | 156 | 526 | 882  | 796  | 374  | 86  | 8   |   |
| 0 | 0 | 0 | 0 | 0 | 24 | 186 | 544 | 756  | 532  | 198  | 36  | 2   |   |
| 0 | 0 | 0 | 0 | 0 | 12 | 144 | 654 | 1441 | 1694 | 1083 | 362 | 58  | 4 |
| 0 | 0 | 0 | 0 | 0 | 15 | 153 | 597 | 1109 | 1048 | 506  | 119 | 11  |   |
| 0 | 0 | 0 | 0 | 0 | 12 | 99  | 312 | 460  | 326  | 121  | 22  | 1   |   |
| 0 | 0 | 0 | 0 | 0 | 9  | 120 | 587 | 1376 | 1732 | 1218 | 469 | 89  | 6 |
| 0 | 0 | 0 | 0 | 0 | 15 | 138 | 495 | 873  | 812  | 395  | 91  | 7   |   |
| 0 | 0 | 0 | 0 | 0 | 21 | 174 | 555 | 860  | 694  | 297  | 63  | 5   |   |
| 0 | 0 | 0 | 0 | 0 | 9  | 132 | 655 | 1459 | 1650 | 1020 | 347 | 60  | 4 |
| 0 | 0 | 0 | 0 | 0 | 9  | 87  | 323 | 564  | 488  | 220  | 49  | 4   |   |
| 0 | 0 | 0 | 0 | 0 | 12 | 90  | 252 | 337  | 236  | 88   | 16  | 1   |   |
| 0 | 0 | 0 | 0 | 0 | 12 | 123 | 498 | 1017 | 1146 | 725  | 246 | 39  | 2 |
| 0 | 0 | 0 | 0 | 0 | 15 | 138 | 495 | 873  | 812  | 395  | 91  | 7   |   |
| 0 | 0 | 0 | 0 | 0 | 12 | 90  | 252 | 337  | 236  | 88   | 16  | 1   |   |
| 0 | 0 | 0 | 0 | 0 | 12 | 135 | 584 | 1232 | 1398 | 888  | 314 | 57  | 4 |
| 0 | 0 | 0 | 0 | 0 | 9  | 87  | 323 | 564  | 488  | 220  | 49  | 4   |   |
| 0 | 0 | 0 | 0 | 0 | 0  | 3   | 20  | 41   | 30   | 11   | 2   |     |   |
| 0 | 0 | 0 | 0 | 0 | 15 | 183 | 827 | 1768 | 1974 | 1195 | 389 | 63  | 4 |
| 0 | 0 | 0 | 0 | 0 | 18 | 171 | 626 | 1087 | 946  | 429  | 96  | 8   |   |
| 0 | 0 | 0 | 0 | 0 | 18 | 186 | 756 | 1541 | 1722 | 1063 | 356 | 60  | 4 |
| 0 | 0 | 0 | 0 | 0 | 21 | 174 | 555 | 860  | 694  | 297  | 63  | 5   |   |
| 0 | 0 | 0 | 0 | 0 | 18 | 186 | 738 | 1409 | 1388 | 702  | 166 | 13  |   |
| 0 | 0 | 0 | 0 | 0 | 18 | 171 | 626 | 1087 | 946  | 429  | 96  | 8   |   |
| 0 | 0 | 0 | 0 | 0 | 18 | 207 | 882 | 1758 | 1770 | 891  | 216 | 21  |   |
| 0 | 0 | 0 | 0 | 0 | 18 | 171 | 636 | 1173 | 1152 | 591  | 138 | 9   |   |
| 0 | 0 | 0 | 0 | 0 | 18 | 162 | 566 | 964  | 856  | 396  | 90  | 8   |   |
| 0 | 0 | 0 | 0 | 0 | 12 | 96  | 292 | 419  | 296  | 110  | 20  | 1   |   |
| 0 | 0 | 0 | 0 | 0 | 15 | 168 | 725 | 1532 | 1738 | 1084 | 361 | 59  | 4 |
| 0 | 0 | 0 | 0 | 0 | 15 | 159 | 637 | 1191 | 1108 | 528  | 123 | 11  |   |
| 0 | 0 | 0 | 0 | 0 | 18 | 162 | 566 | 964  | 856  | 396  | 90  | 8   |   |
| 0 | 0 | 0 | 0 | 0 | 12 | 96  | 292 | 419  | 296  | 110  | 20  | 1   |   |
| 0 | 0 | 0 | 0 | 0 | 12 | 165 | 814 | 1891 | 2324 | 1577 | 584 | 109 | 8 |
| 0 | 0 | 0 | 0 | 0 | 18 | 162 | 566 | 964  | 856  | 396  | 90  | 8   |   |
| 0 | 0 | 0 | 0 | 0 | 24 | 183 | 524 | 715  | 502  | 187  | 34  | 2   |   |
| 0 | 0 | 0 | 0 | 0 | 24 | 222 | 798 | 1396 | 1270 | 604  | 138 | 11  |   |
| 0 | 0 | 0 | 0 | 0 | 24 | 222 | 816 | 1528 | 1604 | 965  | 328 | 58  | 4 |
| 0 | 0 | 0 | 0 | 0 | 18 | 216 | 958 | 1982 | 2108 | 1229 | 394 | 64  | 4 |
| 0 | 0 | 0 | 0 | 0 | 24 | 228 | 840 | 1509 | 1416 | 682  | 160 | 15  |   |
| 0 | 0 | 0 | 0 | 0 | 21 | 225 | 911 | 1736 | 1668 | 814  | 193 | 18  |   |
| 0 | 0 | 0 | 0 | 0 | 24 | 213 | 738 | 1273 | 1180 | 571  | 132 | 11  |   |
| 0 | 0 | 0 | 0 | 0 | 24 | 183 | 524 | 715  | 502  | 187  | 34  | 2   |   |



|   |   |   |   |   |    |     |     |      |      |      |     |     |   |
|---|---|---|---|---|----|-----|-----|------|------|------|-----|-----|---|
| 0 | 0 | 0 | 0 | 0 | 21 | 210 | 827 | 1632 | 1766 | 1064 | 355 | 61  | 4 |
| 0 | 0 | 0 | 0 | 0 | 21 | 180 | 595 | 942  | 754  | 319  | 67  | 5   |   |
| 0 | 0 | 0 | 0 | 0 | 21 | 210 | 809 | 1500 | 1432 | 703  | 165 | 14  |   |
| 0 | 0 | 0 | 0 | 0 | 21 | 180 | 595 | 942  | 754  | 319  | 67  | 5   |   |
| 0 | 0 | 0 | 0 | 0 | 18 | 207 | 898 | 1859 | 2018 | 1196 | 388 | 64  | 4 |
| 0 | 0 | 0 | 0 | 0 | 21 | 180 | 595 | 942  | 754  | 319  | 67  | 5   |   |
| 0 | 0 | 0 | 0 | 0 | 12 | 186 | 956 | 2209 | 2620 | 1710 | 616 | 113 | 8 |
| 0 | 0 | 0 | 0 | 0 | 18 | 168 | 606 | 1046 | 916  | 418  | 94  | 8   |   |
| 0 | 0 | 0 | 0 | 0 | 24 | 180 | 504 | 674  | 472  | 176  | 32  | 2   |   |
| 0 | 0 | 0 | 0 | 0 | 18 | 192 | 796 | 1623 | 1782 | 1085 | 360 | 60  | 4 |
| 0 | 0 | 0 | 0 | 0 | 18 | 168 | 606 | 1046 | 916  | 418  | 94  | 8   |   |
| 0 | 0 | 0 | 0 | 0 | 30 | 249 | 798 | 1260 | 1062 | 473  | 104 | 9   |   |
| 0 | 0 | 0 | 0 | 0 | 24 | 243 | 940 | 1714 | 1566 | 737  | 170 | 15  |   |
| 0 | 0 | 0 | 0 | 0 | 24 | 243 | 940 | 1714 | 1566 | 737  | 170 | 15  |   |
| 0 | 0 | 0 | 0 | 0 | 24 | 243 | 940 | 1714 | 1566 | 737  | 170 | 15  |   |
| 0 | 0 | 0 | 0 | 0 | 24 | 234 | 880 | 1591 | 1476 | 704  | 164 | 15  |   |
| 0 | 0 | 0 | 0 | 0 | 24 | 189 | 564 | 797  | 562  | 209  | 38  | 2   |   |
| 0 | 0 | 0 | 0 | 0 | 36 | 270 | 756 | 1011 | 708  | 264  | 48  | 3   |   |

## Theorem 3

We define the SLACK function (equation (10) ) we use to prove Theorem 3.

```
Slack4[λ_, Δ0_, Δ1_, Δ2_, CC_] :=
  AlpV[CC, λ] - αP52[λ] - Δ0 * ( GamV[CC, λ, 0] - GamU[CC, λ, 0] ) -
  Δ1 * ( GamV[CC, λ, 1] - GamU[CC, λ, 1] ) - Δ2 * ( GamV[CC, λ, 2] - GamU[CC, λ, 2] )
```

Here we rescale the slack function by multiplying it with the Petersen partition function and the configuration partition function (both polynomials with positive coefficients).

```
In[23]:= ScaledSlack4[λ_, Δ0_, Δ1_, Δ2_, CC_] := PP52[λ] * ZZ[CC, λ] * Slack4[λ, Δ0, Δ1, Δ2, CC]
```

## Claim 12

We set values of the dual variables for  $\lambda$  in  $[0, 3/16]$ , as in Claim 12 and define the function  $\lambda[t]$  for this range.

```
In[24]:= L1r0[λ_] := - ( ( 3 ( λ2 + 10 λ3 + 38 λ4 + 67 λ5 + 57 λ6 + 21 λ7 + 4 λ8 ) ) /
  ( ( 1 + 7 λ + 11 λ2 + 10 λ3 + 4 λ4 ) ( 1 + 10 λ + 30 λ2 + 30 λ3 + 5 λ4 ) ) );
L2r0[λ_] := - ( ( 3 ( λ2 + 9 λ3 + 33 λ4 + 64 λ5 + 68 λ6 + 31 λ7 + 4 λ8 ) ) /
  ( ( 1 + 7 λ + 11 λ2 + 10 λ3 + 4 λ4 ) ( 1 + 10 λ + 30 λ2 + 30 λ3 + 5 λ4 ) ) );
λ12[t_] := 3 / 16 * t / (1 + t);
```

Loop over all configurations and print a scaling of ScaledSlack4 by the factor  $(17592186044416(1+t)^{11}(16384 + 87040t + 169152t^2 + 143800t^3 + 45385t^4))$ , which is positive for all  $t > 0$ . We plug in  $\lambda[t]$  and calculate the coefficients of the resulting polynomial in  $t$ . We find either that the polynomial is identically 0 or we report the minimum coefficient. Claim 12 is proved by noting that the minimum coefficient is always  $\geq 0$ .

```

CoefListTable1 = Table[{}, {i, 1, Length[CONFIGURATIONS4]};
For[i = 1, i ≤ Length[CONFIGURATIONS4], i++, SSLack = Simplify[
  (17592186044416 (1 + t)11 (16384 + 87040 t + 169152 t2 + 143800 t3 + 45385 t4)) *
  ScaledSlack4[λ, 0, L1r0[λ], L2r0[λ], CONFIGURATIONS4[[i]]] /. λ → (λ12[t])];
(*Print["Scaled slack function: ", SSLack];*)
CoefList = CoefficientList[SSLack, t];
CoefListTable1[[i]] = CoefList;
(*Print[CoefList];*)
If[CoefList == {}, Print["Config: ", i, " Identically 0"]];
]

```

Config: 78 Identically 0

Config: 79 Identically 0

Config: 80 Identically 0

Check to see if there are any negative coefficients.

```
Min[Flatten[CoefListTable1]]
```

0

Run the command below so see all coefficients (large output).

```
Print[CoefListTable1]
```

## Claim 13

We set values of the dual variables for  $\lambda$  in  $[3/16, 11/20]$ , as in Claim 13 and define the function  $\lambda[t]$  for this range.

$$\text{In[27]:= } L1r1[\lambda_-] := \frac{-6\lambda^2 - 36\lambda^3 - 75\lambda^4 - 64\lambda^5 - 13\lambda^6 + 4\lambda^7}{2(1 + 12\lambda + 52\lambda^2 + 111\lambda^3 + 135\lambda^4 + 100\lambda^5 + 40\lambda^6 + 5\lambda^7)};$$

$$L2r1[\lambda_-] := \frac{-3\lambda^2 - 21\lambda^3 - 49\lambda^4 - 45\lambda^5 - 6\lambda^6}{2(1 + \lambda + \lambda^2)(1 + 10\lambda + 30\lambda^2 + 30\lambda^3 + 5\lambda^4)};$$

$$\lambda13[t_-] := 11/20 * (3/16 * 20 / (11 + t)) / (1 + t);$$

Loop over all configurations and print a scaling of ScaledSlack4

by the factor  $(1 + t)^{12} (95 + 124t) (7825 + 18840t + 11856t^2)$ ,

which is positive for all  $t > 0$ . We plug in  $\lambda[t]$  and calculate the coefficients of the resulting polynomial in  $t$ . We find either that the polynomial is identically 0 or we report the minimum coefficient. Claim 13 is proved by noting that the minimum coefficient is always  $\geq 0$ .

```

CoefListTable2 = Table[{}, {i, 1, Length[CONFIGURATIONS4]};
For[i = 1, i ≤ Length[CONFIGURATIONS4], i++,
  SSLack = Simplify[(1 + t)12 (95 + 124 t) (7825 + 18840 t + 11856 t2) *
    ScaledSlack4[λ, 0, L1r1[λ], L2r1[λ], CONFIGURATIONS4[[i]]] /. λ → (λ13[t])];
  (*Print["Scaled slack function: ", SSLack];*)
  CoefList = CoefficientList[SSLack, t];
  CoefListTable2[[i]] = CoefList;
  (*Print[CoefList];*)
  If[CoefList == {}, Print["Config: ", i, " Identically 0"]];
]

```

```

Config: 25  Identically 0
Config: 78  Identically 0
Config: 79  Identically 0
Config: 130 Identically 0

```

Check to see if there are any negative coefficients.

```
Min[Flatten[CoefListTable2]]
```

```

11 209 195 125
536 870 912

```

Run the command below so see all coefficients (large output).

```
Print[CoefListTable2];
```

## Claim 14

We set values of the dual variables for  $\lambda$  in  $[11/20, \text{Sqrt}[3/5]]$ , as in Claim 14 and define the function  $\lambda[t]$  for this range.

```

In[30]:= L1r3[λ_] := 
$$\frac{-6 \lambda^2 - 42 \lambda^3 - 111 \lambda^4 - 125 \lambda^5 - 41 \lambda^6 + 5 \lambda^7}{2 (1 + 13 \lambda + 63 \lambda^2 + 152 \lambda^3 + 205 \lambda^4 + 165 \lambda^5 + 75 \lambda^6 + 10 \lambda^7)};$$

L2r3[λ_] := 
$$\frac{-3 \lambda^2 - 24 \lambda^3 - 83 \lambda^4 - 140 \lambda^5 - 96 \lambda^6 - 12 \lambda^7}{2 (1 + 3 \lambda + 3 \lambda^2 + 2 \lambda^3) (1 + 10 \lambda + 30 \lambda^2 + 30 \lambda^3 + 5 \lambda^4)};$$

λ14[t_] := Sqrt[3 / 5] * (11 / 20 * Sqrt[5 / 3] + t) / (1 + t)

```

Loop over all configurations and print

```

a scaling of ScaledSlack4 by the factor (1 + t)11
(15 561 + 6 (4805 + 1082 √15) t + 120 (281 + 62 √15) t2 + 1120 (10 + 3 √15) t3)
(10 468 833 921 + 6 (6 854 491 225 + 1 948 781 218 √15) t +
360 (419 372 049 + 110 874 710 √15) t2 + 800 (374 453 440 + 96 980 607 √15) t3 +
64 000 (5 517 557 + 1 426 590 √15) t4 + 5 145 600 (48 675 + 12 484 √15) t5 +
1 024 000 (95 362 + 24 765 √15) t6 + 28 672 000 (575 + 148 √15) t7),

```

which is positive for all  $t > 0$ . We plug in  $\lambda[t]$  and calculate the coefficients of the resulting polynomial in  $t$ . We find either that the polynomial is identically 0 or we report the minimum coefficient. Claim 14 is proved by noting that the minimum coefficient is always  $\geq 0$ .

```

CoefListTable3 = Table[{}, {i, 1, Length[CONFIGURATIONS4]};
For[i = 1, i ≤ Length[CONFIGURATIONS4], i++, SSlack = Simplify[
  (1 + t)11 (15 561 + 6 (4805 + 1082 √15) t + 120 (281 + 62 √15) t2 + 1120 (10 + 3 √15) t3)
  (10 468 833 921 + 6 (6 854 491 225 + 1 948 781 218 √15) t +
    360 (419 372 049 + 110 874 710 √15) t2 + 800 (374 453 440 + 96 980 607 √15) t3 +
    64 000 (5 517 557 + 1 426 590 √15) t4 + 5 145 600 (48 675 + 12 484 √15) t5 +
    1 024 000 (95 362 + 24 765 √15) t6 + 28 672 000 (575 + 148 √15) t7) *
  ScaledSlack4[λ, 0, L1r3[λ], L2r3[λ], CONFIGURATIONS4[[i]]] /. λ → (λ14[t]);
CoefList = CoefficientList[SSlack, t];
CoefListTable3[[i]] = CoefList;
(*Print[CoefList];*)
If[CoefList == {}, Print["Config: ", i, " Identically 0"]];
]

```

Config: 7 Identically 0

Config: 25 Identically 0

Config: 79 Identically 0

Config: 88 Identically 0

Config: 130 Identically 0

Config: 181 Identically 0

Check to see if there are any negative coefficients.

```

Min[Flatten[CoefListTable3]]
15 222 350 434 666 986 471 861
5 120 000 000

```

Run the command below to see all coefficients (large output).

```
Print[CoefListTable3];
```

## Claim 15

We set values of the dual variables for  $\lambda$  in  $[\text{Sqrt}[3/5], 1]$ , as in Claim 15 and define the function  $\lambda[t]$  for this range

```

In[33]:= L0r4[λ_] := 
$$\frac{-3 - 30\lambda - 117\lambda^2 - 196\lambda^3 - 88\lambda^4 + 86\lambda^5 + 66\lambda^6 + 12\lambda^7}{6\lambda(1+\lambda)^2(1+10\lambda+30\lambda^2+30\lambda^3+5\lambda^4)};$$

L1r4[λ_] := 
$$\frac{-3 - 27\lambda - 87\lambda^2 - 118\lambda^3 - 54\lambda^4 - 3\lambda^5 - 18\lambda^6}{6\lambda(1+\lambda)(1+10\lambda+30\lambda^2+30\lambda^3+5\lambda^4)};$$

L2r4[λ_] := 
$$\frac{-3 - 30\lambda - 105\lambda^2 - 160\lambda^3 - 100\lambda^4 - 18\lambda^5 - 6\lambda^6}{6\lambda(1+\lambda)(1+10\lambda+30\lambda^2+30\lambda^3+5\lambda^4)}$$

λ15[t_] := (t + Sqrt[3/5]) / (t + 1)

```

Loop over all configurations and print a scaling

of ScaledSlack4 by the factor  $(1 + t)^{11} (5 + \sqrt{15} + 10t)$ ,

which is positive for all  $t > 0$ . We plug in  $\lambda[t]$  and calculate the

coefficients of the resulting polynomial in  $t$ . We find either that the

polynomial is identically 0 or we report the minimum coefficient. Claim 15 is proved by noting that the minimum coefficient is always  $\geq 0$ .

```
CoefListTable4 = Table[{}, {i, 1, Length[CONFIGURATIONS4] }];
For[i = 1, i ≤ Length[CONFIGURATIONS4], i++,
  SSLack = Simplify[(1 + t)11 (5 + √15 + 10 t) * ScaledSlack4[λ,
    L0r4[λ], L1r4[λ], L2r4[λ], CONFIGURATIONS4[[i]]] /. λ → (λ15[t])];
  (*Print["Scaled slack function: ", SSLack];*)
  CoefList = CoefficientList[SSLack, t];
  CoefListTable4[[i]] = CoefList;
  (*Print[CoefList];*)
  If[CoefList == {}, Print["Config: ", i, " Identically 0"]];
]
```

Config: 7 Identically 0

Config: 44 Identically 0

Config: 58 Identically 0

Config: 73 Identically 0

Config: 79 Identically 0

Config: 88 Identically 0

Config: 95 Identically 0

Config: 162 Identically 0

Config: 181 Identically 0

Config: 193 Identically 0

Config: 201 Identically 0

Check to see if there are any negative coefficients.

```
Min[Flatten[CoefListTable4]]
```

0

Run the command below to see all coefficients (large output).

```
Print[CoefListTable3];
```
